# Supplementary material for: A General Graph Spectral Wavelet Convolution via Chebyshev Order Decomposition
Source: arXiv:2405.13806 source file (2025-05-14)
Supplement: Supplementary file 1 [file matrix.tex]

\section{Relationship between Graph Convolution and Transformer}
\label{relation}
To recap, the vanilla Transformer~\citep{va_trans} is given as:
\begin{equation}
\label{generall}
    \bm{H}^{(l+1)}=\textrm{softmax}\left(\frac{\bm{H}^{(l)}\bm{W}_q(\bm{H}^{(l)}\bm{W}_k)^\top}{\sqrt{d}}\right)\bm{H}^{(l)}\bm{W}_v,
\end{equation}
where $\bm{H}^{(l)}, \bm{H}^{(l+1)}\in\mathbb{R}^{N\times d}$ are node embeddings from $l$th and ($l+1$)th layers, and $\{\bm{W}_q, \bm{W}_k, \bm{W}_v\}\in\mathbb{R}^{d\times d}$ are the query, key, and value learnable matrices. This self-attention mechanism can be written as a kernel summation in the discrete case~\citep{mialon2021graphit, tsai2019transformer,afno}. Specifically for node $s$, $\bm{h}^{(l+1)}_s=\sum\limits_t \bm{\kappa}(s,t)\bm{h}^{(l)}_t$, where $\bm{\kappa}(s,t)=\textrm{softmax}(\frac{\bm{H}^{(l)}\bm{W}_q(\bm{H}^{(l)}\bm{W}_k)^\top}{\sqrt{d}})_{(s,t)}\cdot \bm{W}_v$. Therefore, $\bm{\kappa}: \{1,\dots, N\}\times\{1,\dots, N\}\rightarrow\mathbb{R}^{d\times d}$ is treated as an asymmetric matrix-valued kernel. Note that the usage of asymmetric kernel is also commonly used in various machine learning tasks~\citep{kulis2011you}. Further assume $\bm{\kappa}(s,t)=\bm{\kappa}(s-t)$, which indicates a shift-invariant GT since the attention depends on the difference between two nodes rather than their positions. Then, Eq.~(\ref{generall}) becomes a convolution $\bm{h}^{(l+1)}_s=\sum\limits_t \bm{\kappa}(s-t)\bm{h}^{(l)}_t$, which can be expressed with the convolution theorem as:
\begin{equation}
\label{sadaseqrqrr}
    \bm{h}^{(l+1)}_s=\mathcal{F}^{-1}(\mathcal{F}(\bm{\kappa})\cdot\mathcal{F}(\bm{H}^{(l)}))(s)\in\mathbb{R}^{1\times d}.
\end{equation}
Eq.~(\ref{sadaseqrqrr}) is also known as Fourier integral operator~\citep{hormander1971fourier}. In Eq.~(\ref{sadaseqrqrr}), for each frequency mode $n\in N$ (i.e., $\mathcal{F}(\bm{H}^{(l)})(n, \cdot)$), $\mathcal{F}(\bm{\kappa})(n)\in\mathbb{R}^{d\times d}$, because $\bm{\kappa}: \{1,\dots, N\}\times\{1,\dots, N\}\rightarrow\mathbb{R}^{d\times d}$. Hence, for all modes, $\mathcal{F}(\bm{\kappa})$ can be fully parameterized by a neural network $R_\theta\in\mathbb{R}^{N\times d\times d}$~\citep{fno}:
\begin{equation}
\label{fnofnoo}
    \bm{h}^{(l+1)}_s=\mathcal{F}^{-1}(R_\theta\cdot\mathcal{F}(\bm{H}^{(l)}))(s)\in\mathbb{R}^{1\times d}.
\end{equation}
